# Supplementary material for: Diffusion Models for Generative Outfit Recommendation
Source: arXiv:2402.17279 source file (2024-05-20)
Supplement: Supplementary file 1 [file 6_SI.tex]

\section{Appendix}
\label{sec:appendix}
